# Supplementary material for: From Human Bias to Robot Choice: How Occupational Contexts and Racial Priming Shape Robot Selection
Source: arXiv:2512.20951 source file (2026-01-16)
Supplement: Supplementary file 1 [file appendix.pdf]

# A Robot Stimuli

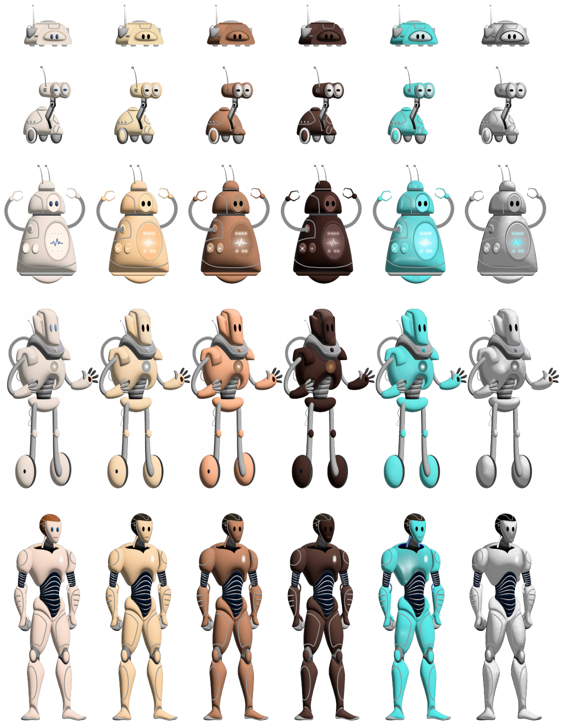

**Figure 7: Robot stimuli used in the study, including the baseline robots (silver and teal), and the robots with four different skin tones in five different human-likeness levels.**

# B Survey Questions

## B.1 Task Scenarios

- **Task 1: Robot Selection for a Construction Site**
  In this setting, the selected robot will assist in managing a construction site. The robot will be responsible for operating machinery, overseeing the worksite, coordinating the project, and ensuring the safety of workers.
- **Task 2: Robot Selection for Home Tutoring**
  In this home tutoring setting, the selected robot will be responsible for providing personalized tutoring for students. The robot will deliver lessons, answer questions, and assist with assignments. The ideal robot should have the ability to explain complex topics clearly and help with study planning.
- **Task 3: Robot Selection for a Hospital Setting**
  In this hospital setting, the selected robot will play a key role in providing emotional support and simple healthcare services to patients. The robot will offer companionship and healthcare during recovery, engage in conversations to reduce feelings of loneliness and anxiety, and assist in the general emotional well-being of patients.
- **Task 4: Robot Selection for a Sports Field Task**
  In this sports field setting, the selected robot will oversee practices, provide feedback on athlete performance, and help design training regimens. The robot should be able to plan workout routines and encourage athletes to perform at their best.

## B.2 Task-Specific Attitudes

- How helpful do you believe robots are in assisting with tasks in a construction site/home tutoring setting/hospital/sports filed? (1: Not at all helpful, 7: Very helpful)
- How concerned are you that robots may replace human workers in construction roles/home tutore roles/emotional support roles/assisting athletes roles in the future? (1: Not at all concerned, 7: Very concerned)
- How important do you think it is for robots to have a human-like appearance while performing tasks on a sports field/home tutoring setting/hospital/construction site? (1: Not at all important, 7: Very important)

## B.3 Robot and AI Attitudes

- How much did the robot's colors influence your task selection? (1: Not at all, 7: Very much)
- How comfortable are you with the idea of interacting with robots in your daily life? (1: Not at all, 11: Very much)
- What is your general opinion of Artificial Intelligence (AI) technologies (e.g., ChatGPT, AI-based robot)? (1: Very negative, 12: Very positive)
- Thinking about all robots you just saw (with different colors but the same design), how human-like do you think these robots appear overall?
  Please rate from 1 (not human-like at all) to 7 (very human-like) using the reference images below as a guide.

# C Robot Color Preferences by Human-likeness

The standard deviations (Std) represent the mean of the percentage differentiation between the four skin-tone colors. The table demonstrates the pattern we observed in Figure 3: the moderate human-likeness level (=3) intensifies preferences for human-like appearances in most contexts. Another interesting pattern is that the percentage differentiation between skin-tone colors becomes smaller when human-likeness level is high, but the increase is not linear.

# D Limitations and Future Research

First, our participants were based in the United States, and both occupational stereotypes and racialized role expectations can vary across cultural contexts. Therefore, our inferences are constrained to the United States context, and cross-cultural replications are needed to assess whether these patterns generalize or take different forms elsewhere. Second, our scenarios were hypothetical rather than embedded in real deployment settings, which may under- or over-estimate the strength of selection biases in practice. Third, we focused on skin tone while controlling other appearance cues, which clarifies interpretation but does not capture how multiple identity-relevant cues may interact in real robot designs. Fourth, we

**Table 4: Robot color preferences by human-likeness and task. Frequencies for baseline vs skin-tone options with standard deviations for skin-tone colors.**

| CONSTRUCTION | | | | TUTORING | | | |
|---|---|---|---|---|---|---|---|
| H | Baseline | Skin | Std | H | Baseline | Skin | Std |
| 1 | 56.6% | 43.4% | 5.8% | 1 | 59.0% | 41.0% | 9.1% |
| 2 | 45.5% | 54.5% | 6.1% | 2 | 52.3% | 47.7% | 7.1% |
| 3 | 58.0% | 42.0% | 4.3% | 3 | 46.9% | 53.1% | 10.3% |
| 4 | 51.2% | 48.8% | 5.2% | 4 | 51.2% | 48.8% | 6.1% |
| 5 | 51.8% | 48.2% | 5.7% | 5 | 65.9% | 34.1% | 6.2% |
| *m* | 52.6% | 47.4% | 5.4% | *m* | 55.1% | 44.9% | 7.8% |
| **HOSPITAL** | | | | **SPORTS** | | | |
| H | Baseline | Skin | Std | H | Baseline | Skin | Std |
| 1 | 48.2% | 51.8% | 8.1% | 1 | 53.0% | 47.0% | 5.1% |
| 2 | 40.7% | 59.3% | 9.5% | 2 | 46.6% | 53.4% | 6.9% |
| 3 | 32.1% | 67.9% | 14.8% | 3 | 46.9% | 53.1% | 4.0% |
| 4 | 48.8% | 51.2% | 7.1% | 4 | 41.7% | 58.3% | 8.0% |
| 5 | 55.3% | 44.7% | 7.5% | 5 | 55.3% | 44.7% | 3.4% |
| *m* | 45.0% | 55.0% | 9.4% | *m* | 48.7% | 51.3% | 5.5% |

relied on rendered robot illustrations rather than physical robots, which strengthens experimental control but may not fully capture how materials, motion, and embodiment cues influence selection in real-world HRI. Future work should test interventions in more ecologically valid deployments, vary multiple appearance and embodiment cues jointly, and replicate the paradigm across cultural settings.

Received 20 February 2007; revised 12 March 2009; accepted 5 June 2009
